# Supplementary material for: Stable long-range uniaxial order in active fluids at two-dimensional interfaces
Source: arXiv:2010.15044 ancillary file (2021-02-25)
Supplement: Supplementary file 1 [file film_nem_supp.pdf]

# Stable long-range uniaxial order in active fluids at two-dimensional interfaces: Supplementary Material

Ananyo Maitra[1, *]

[1] *Sorbonne Université and CNRS, Laboratoire Jean Perrin, F-75005, Paris, France*

In this supplement I present the calculations for the main paper. Sec I presents the calculation for a two-dimensional nematic state at an interface between two fluids in which the number of active units is not conserved. Sec. II discusses a nematic state in which the number of active units is conserved. Sec. III presents a discussion of a polar state. Finally, Sec. IV explicitly considers the effect of interfacial height fluctuations on the tangent plane order.

## I. ACTIVE NEMATICS AT THE INTERFACE BETWEEN TWO FLUIDS

In this section I will present the detailed calculations for the a two-dimensional apolar ordered phase at a thin, perfectly flat interfacial layer at $z = 0$ immersed in an incompressible fluid. Implicitly averaging over the small thickness of the interfacial layer, I will consider the effectively two-dimensional dynamics of the ordered phase on a surface or interface immersed in a three-dimensional fluid.

As discussed in the main text, I will consider the fluid above and below the interface to be viscosity matched. I will also consider the dynamics of the layer at scales much larger than the Saffman-Delbrück scale [17, 23]. Below this scale, the momentum is essentially confined to the two-dimensional film and above this scale, the momentum-exchange with the three-dimensional medium becomes important. Scales larger than the Saffman-Delbrück scale are relevant for experiments on motor-microtubule experiments at interfaces [8] as can be seen from the following argument: below the Saffman-Delbrück scale, the active layer behaves as a two-dimensional momentum-conserved fluid and if that were the relevant scale, would have suffered a Simha-Ramaswamy instability [6, 8] with a fastest growing mode at zero wavenumber. This is not what is observed in experiments on motor-microtubule layers [8] where it is possible to identify a fastest growing mode at a non-zero wavenumber. The growth-rate being maximal at a non-zero wavenumber is a clear signature of momentum exchange with the bulk, three-dimensional fluid medium and implies that the relevant scale in these experiments is larger than the Saffman-Delbrück length. This is also likely to be the case for other realisations of active ordered phases at interfaces, for instance, formed by bacteria at a two fluid interface or ordering associated with cell membranes or artificial biomimetic realisations.

In this first section, I consider nematic ordering at an interface in a situation in which the number of nematogens *at the interface* is not conserved but is locally constant on average. This *does not* imply that the *total* number of nematogens is not conserved or that the total mass is not conserved. The density of the nematogens (or monomers composing the nematogens) is taken to be conserved in *three* dimensions.

### A. Density non-conservation in the layer

The three-dimensional, conserved density of the nematogens is denoted by $\rho$. I take the density field to be controlled by a free energy $F_\rho$ and assume that it favours an inhomogeneous density profile with the density highest at the interface. The conservation of the nematogen concentration $\rho$ in three dimensions has the form

$$\partial_t \rho = -\nabla \cdot (\mathbf{V}\rho) + D_3 \nabla^2 \frac{\delta F_\rho}{\delta \rho} \tag{1}$$

where $\mathbf{V}$ is the bulk, three-dimensional fluid velocity, which is taken to be incompressible i.e., $\nabla \cdot \mathbf{V} = 0$. The effect on the three-dimensional velocity field due to the three-dimensional conserved density is accounted for via the three-dimensional force-balance equation

$$\eta \nabla^2 \mathbf{V} = \nabla \Pi + \rho \nabla \frac{\delta F_\rho}{\delta \rho} + \mathbf{f}_{\text{int}} \delta(z) \tag{2}$$

where $\Pi$ is the three-dimensional pressure that enforces the constraint of incompressibility, the second term arises as a consequence of Onsager symmetry and the $\mathbf{f}_{\text{int}}\delta(z)$ contain interfacial forces to be discussed in the next subsection. If the dynamics of $\rho$ is fast enough compared to the timescale of the interfacial dynamics, such that the three-dimensional density field relaxes to its steady state value given by $\delta F_\rho / \delta \rho = 0$ effectively instantaneously in that timescale, then

we can ignore the dynamics of the three-dimensional conserved density field of the nematogens while considering their in-plane dynamics. Further, this argument remains valid even when the $z-$dependent inhomogeneous density profile is maintained by an active mechanism, as in active Brownian particles or bacterial fluids. Furthermore, even if the constraint of fast relaxation is relaxed, the density field is likely to be a purely $z-$dependent function which is symmetric about $z = 0$. Therefore, by symmetry, it cannot lead to in-plane flows at $z = 0$ and therefore, cannot affect interfacial ordering. This situation is relevant, for instance, for interfacial ordering of bacterial fluids.

A somewhat different situation arises when the number of monomers composing the nematogenic particles is conserved in three dimensions, but they associate (and dissociate) to form nematogenic units only at the interface. This situation is relevant for cortical membrane associated ordering in cells [7]. It may be achieved in experiments on motor-microtubule films [8, 22] if an association-dissociation protocol is implemented at the interface, as pointed out in the main text. In this case, $\rho$ denotes the three-dimensional *monomeric* concentration (including both free monomers as well as those in the nematogenic filaments) while $\rho_N$ denotes the density of the nematogens at the interface. Since they associate and dissociate at the interface, the concentration of the nematogens has an equation of motion

$$\dot{\rho}_N = -k_1\rho_N + k_0\rho(z=0) \tag{3}$$

to lowest order in gradients. If this association-dissociation rate is fast-enough, $\rho_N$ can be taken to be fixed at an average value $\langle\rho_N\rangle = k_0\langle\rho(z=0)\rangle/k_1$. The concentration $\rho$ (i.e., the concentration of monomers) can be taken to be homogeneous in three dimensions and $\langle\rho_N\rangle$ can be set to 1 without loss of generality. The dynamics of $\rho$ is still governed by (1) and (2). In this case, since the steady-state distribution of $\rho$ can be assumed to be homogeneous in three dimensions, linear deviations from it only modify the three-dimensional pressure and does not lead to flows. Since the dynamics of the in-plane order depends on in-plane flows at $z = 0$, they cannot be affected by the three-dimensional density field (to lowest order in gradients) even in this case.

### B. Model specification and analysis

I now define the variables of my model ignoring the dynamics of the three-dimensional density field (which, as discussed above, doesn't affect the dynamics of in-plane order and can be absorbed in the pressure at least in the second case considered above). The three-dimensional bulk fluid velocity $\mathbf{V}(\mathbf{r},t) \equiv \mathbf{V}(\mathbf{r}_\perp, z, t)$, where $\mathbf{r}_\perp \equiv (x, y)$, is incompressible i.e., $\nabla\cdot\mathbf{V} = 0$. The two dimensional nematic order, which is taken to be along $\hat{x}$, is described by the two-dimensional apolar order parameter

$$\mathsf{Q} = \frac{S}{2}\begin{pmatrix}\cos 2\theta & \sin 2\theta \\ \sin 2\theta & -\cos 2\theta\end{pmatrix} \tag{4}$$

where $\theta$ is the deviation of the local nematic order from $\hat{x}$ and $S$ is the magnitude of the nematic order whose steady state value is $S_0 = \langle S\rangle$. The standard Landau-de Gennes free energy for a two-dimensional nematic is

$$F_Q = \int d\mathbf{r}_\perp \left[\frac{\alpha}{2}(\mathsf{Q}:\mathsf{Q}) + \frac{\beta}{2}(\mathsf{Q}:\mathsf{Q})^2 + \frac{K}{2}(\nabla\mathsf{Q})^2\right] = \int d\mathbf{r}_\perp f_Q \tag{5}$$

which supports an orientationally ordered phase for $\alpha < 0$. For an ordered state along $\hat{x}$,

$$\mathsf{Q}_0 = \frac{S_0}{2}\begin{pmatrix}1 & 0 \\ 0 & -1\end{pmatrix} \tag{6}$$

I will consider the stability of this phase due to active flows. For this, I will consider deviations of $S = S_0 + \delta S$ from its steady state value and the angle field $\theta$ from its steady state value of 0. I denote the in-plane velocity at the plane $z = 0$ as $\mathbf{v}(\mathbf{r}_\perp, t) \equiv (v_x, v_y) = \mathbf{V}_\perp(\mathbf{r}_\perp, z=0, t)$ and the out-of-plane velocity at $z = 0$ as $v_z(\mathbf{r}_\perp, t) = \mathbf{V}_z(\mathbf{r}_\perp, z=0, t)$. The dynamics of the in-plane nematic tensor is

$$\partial_t\mathsf{Q} = -\mathbf{v}\cdot\nabla_\perp\mathsf{Q} + \mathsf{Q}\cdot\mathbf{\Omega} - \mathbf{\Omega}\cdot\mathsf{Q} - \bar{\lambda}\mathsf{A} - \lambda_1[\mathsf{Q}\cdot\mathsf{A}]^{ST} - \Gamma\left[\frac{\delta F_Q}{\delta\mathsf{Q}}\right]^{ST} + \boldsymbol{\xi}^Q, \tag{7}$$

where $\mathbf{\Omega} = (1/2)[\nabla_\perp\mathbf{v} - (\nabla_\perp\mathbf{v})^T]$ is the planar vorticity tensor at the interface, $\mathsf{A} = (1/2)[\nabla_\perp\mathbf{v} + (\nabla_\perp\mathbf{v})^T]$ is the planar strain rate tensor at the interface and $\xi$ is a non-conserving noise with the correlation

$$\langle\xi^Q_{ij}(\mathbf{r}_\perp, t)\xi^Q_{kl}(\mathbf{r}'_\perp, t')\rangle = 2\Delta^Q[\delta_{ik}\delta_{jl} + \delta_{il}\delta_{jk} - \delta_{ij}\delta_{kl}]\delta(\mathbf{r}_\perp - \mathbf{r}'_\perp)\delta(t-t'). \tag{8}$$

Note that $\bar{\lambda}$ *does not* vanish at the isotropic nematic transition [1, 2]. The equation for the velocity field is

$$\eta\nabla^2\mathbf{V} = \nabla\Pi + \nabla_\perp \cdot \left[\bar{\zeta}\mathbf{Q} + \bar{\lambda}\frac{\delta F_Q}{\delta\mathbf{Q}} + \left(\mathbf{Q}\cdot\frac{\delta F_Q}{\delta\mathbf{Q}} - \frac{\delta F_Q}{\delta\mathbf{Q}}\cdot\mathbf{Q}\right) + \lambda_1\left(\mathbf{Q}\cdot\frac{\delta F_Q}{\delta\mathbf{Q}} + \frac{\delta F_Q}{\delta\mathbf{Q}}\cdot\mathbf{Q}\right) + \nabla_\perp\mathbf{Q} : \frac{\partial f_Q}{\partial\nabla_\perp\mathbf{Q}}\right]\delta(z) + \boldsymbol{\xi}^v. \tag{9}$$

Now, I rewrite (7) in terms of magnitude $\delta S$ and angular $\theta$ fluctuations by using

$$\partial_t\delta S = \begin{pmatrix}\cos 2\theta & \sin 2\theta\\ \sin 2\theta & -\cos 2\theta\end{pmatrix} : \partial_t\mathbf{Q} \tag{10}$$

$$\partial_t\theta = \frac{1}{2S}\begin{pmatrix}-\sin 2\theta & \cos 2\theta\\ \cos 2\theta & \sin 2\theta\end{pmatrix} : \partial_t\mathbf{Q} \tag{11}$$

The magnitude equation then yields

$$\partial_t\delta S = -\mathbf{v}\cdot\nabla_\perp\delta S - \Gamma\left[-\alpha + \frac{\beta}{2}S^2 - K\nabla_\perp^2\right]S - \frac{\lambda_1 S}{2}(A_{xx} + A_{yy}) - \bar{\lambda}[\cos 2\theta(A_{xx} - A_{yy}) + 2A_{xy}\sin 2\theta] \tag{12}$$

while the angle field equation is

$$\partial_t\theta = \Omega_{xy} - \frac{\bar{\lambda}}{S}\cos 2\theta A_{xy} + \frac{\bar{\lambda}}{2S}\sin 2\theta(A_{xx} - A_{yy}) + \Gamma_\theta K\nabla_\perp^2\theta + \xi, \tag{13}$$

where $\Gamma_\theta = \Gamma/4S_0^2$ and $\langle\xi(\mathbf{r}_\perp, t)\xi(\mathbf{r}'_\perp, t')\rangle = 2\Delta\delta(\mathbf{r}_\perp - \mathbf{r}'_\perp)\delta(t - t')\delta(z)$, where $\Delta = \Delta^Q/4S_0^2$. Defining $S_0 = \sqrt{2|\alpha|/\beta}$ and plugging this back into (12), I find that that $\delta S$ fluctuations have a wavenumber independent relaxation rate $2\Gamma|\alpha|$. Therefore, I take $S = S_0$ and construct a theory only in terms of the hydrodynamic angular fluctuations. The linearised version of (13) is displayed in the main text with the definition $\lambda = \bar{\lambda}/S_0$. Note that $\lambda$ diverges at the isotropic nematic transition [1, 2].

Since $\delta F_Q/\delta\mathbf{Q} \propto \nabla_\perp^2\theta$ when $S = S_0$, the passive tems in (9) are subdominant to the active term $\propto \bar{\zeta}$. Upon ignoring them, I obtain the linearised equation of motion for the velocity field which is

$$\eta\nabla^2\mathbf{V} = \nabla\Pi + \zeta(\partial_y\theta\hat{x} + \partial_x\theta\hat{y})\delta(z) + \boldsymbol{\xi}^v, \tag{14}$$

with $\zeta = \bar{\zeta}S_0$. Now, I need to calculate $\mathbf{v}$. I eliminate the pressure using the transverse projector on the Fourier-transformed version of (14) and calculate the Fourier-transformed in-plane velocities at $z = 0$:

$$v_x = \int_{-\infty}^{\infty}\frac{dq_z}{2\pi}\frac{i\zeta}{\eta q^4}q_y(q_x^2 - q_y^2 - q_z^2)\theta + \int_{-\infty}^{\infty}\frac{dq_z}{2\pi}\frac{1}{\eta q^4}[q_x(\xi_y^v q_y + \xi_z^v q_z) - \xi_x^v(q_y^2 + q_z^2)] = -\frac{i\zeta}{2\eta}\frac{q_y^3}{|q_\perp|^3}\theta + \bar{\xi}_x^v, \tag{15}$$

$$v_y = \int_{-\infty}^{\infty}\frac{dq_z}{2\pi}\frac{i\zeta}{\eta q^4}q_x(q_y^2 - q_x^2 - q_z^2)\theta + \int_{-\infty}^{\infty}\frac{dq_z}{2\pi}\frac{1}{\eta q^4}[q_y(\xi_x^v q_x + \xi_z^v q_z) - \xi_y^v(q_x^2 + q_z^2)] = -\frac{i\zeta}{2\eta}\frac{q_x^3}{|q_\perp|^3}\theta + \bar{\xi}_y^v, \tag{16}$$

and

$$v_z = \int_{-\infty}^{\infty}\frac{dq_z}{2\pi}\frac{2i\zeta}{\eta q^4}q_x q_y q_z\theta + \int_{-\infty}^{\infty}\frac{dq_z}{2\pi}\frac{1}{\eta q^4}[q_z(\xi_x^v q_x + \xi_y^v q_y) - \xi_z^v q_\perp^2] = \bar{\xi}_z^v, \tag{17}$$

where the noises have the correlations

$$\langle\bar{\xi}_x^v(\mathbf{q}_\perp, t)\bar{\xi}_x^v(\mathbf{q}'_\perp, t)\rangle = \frac{2\Delta^v(q_x^2 + 2q_y^2)}{4\eta^2|q_\perp|^3}\delta(\mathbf{q}_\perp + \mathbf{q}'_\perp)\delta(t - t'), \tag{18}$$

$$\langle\bar{\xi}_y^v(\mathbf{q}_\perp, t)\bar{\xi}_y^v(\mathbf{q}'_\perp, t)\rangle = \frac{2\Delta^v(2q_x^2 + q_y^2)}{4\eta^2|q_\perp|^3}\delta(\mathbf{q}_\perp + \mathbf{q}'_\perp)\delta(t - t'), \tag{19}$$

$$\langle\bar{\xi}_x^v(\mathbf{q}_\perp, t)\bar{\xi}_y^v(\mathbf{q}'_\perp, t)\rangle = -\frac{2\Delta^v q_x q_y}{4\eta^2|q_\perp|^3}\delta(\mathbf{q}_\perp + \mathbf{q}'_\perp)\delta(t - t'), \tag{20}$$

$$\langle \bar{\xi}^v_z(\mathbf{q}_\perp, t)\bar{\xi}^v_z(\mathbf{q}'_\perp, t)\rangle = \frac{2\Delta^v}{4\eta^2|q_\perp|}\delta(\mathbf{q}_\perp + \mathbf{q}'_\perp)\delta(t-t'). \tag{21}$$

As expected from symmetry, Eq. (17) shows that the planar angular fluctuations do not lead to any average flow at the interface in the $\hat{z}$ direction. Instead, the $\hat{z}$ component of the velocity field at the interface is purely a spatiotemporally white, zero-mean noise. This implies that $\langle v_z\rangle$ averaged over the noise vanishes, as expected. Eqs.(15) and (16) imply that the in-plane divergence of the in-plane velocity field has a non-zero angle-dependent part

$$i\mathbf{q}_\perp \cdot \mathbf{v}_\perp = \frac{\zeta}{2\eta}\frac{q_x q_y}{|q_\perp|}\theta. \tag{22}$$

Of course, three-dimensional incompressibility implies that

$$\int_{-\infty}^{\infty}\frac{dq_z}{2\pi}iq_z V_z = -\int_{-\infty}^{\infty}\frac{dq_z}{2\pi}\frac{2\zeta}{\eta q^4}q_x q_y q_z^2\theta = -\frac{\zeta}{2\eta}\frac{q_x q_y}{|q_\perp|}\theta \tag{23}$$

as can be directly verified. A similar relation also holds for the noises at the interface as required by the constraint of incompressibility. Importantly, $i\mathbf{q}_\perp \cdot \mathbf{v}_\perp \neq 0$ directly leads to the existence of a long-range ordered nematic phase.

Plugging the expressions for $v_x$ and $v_y$ back into the angle field equation,

$$\partial_t\theta = -\frac{\zeta}{4\eta}\frac{q_x^4(\lambda-1)+q_y^4(\lambda+1)}{|q_\perp|^3} + \bar{\xi} + \xi = -\kappa(\mathbf{q}_\perp)\theta + \bar{\xi} + \xi \tag{24}$$

where $\bar{\xi}$ is the noise from the velocity field which has the correlation

$$\langle \bar{\xi}(\mathbf{q}_\perp, t)\bar{\xi}(\mathbf{q}'_\perp, t)\rangle = \frac{2\Delta^v[q_x^4(\lambda-1)^2 + q_y^4(\lambda+1)^2 + 2q_x^2q_y^2]}{8\eta^2|q_\perp|^3}\delta(\mathbf{q}_\perp + \mathbf{q}'_\perp)\delta(t-t') \sim \mathcal{O}(q_\perp) \tag{25}$$

Since this vanishes at small $q_\perp$, in all directions, it is subdominant to the non-conserving noise in the angle field $\xi$ (which has the correlation $\langle\xi(\mathbf{r}_\perp, t)\xi(\mathbf{r}'_\perp, t')\rangle = 2\Delta\delta(\mathbf{r}_\perp - \mathbf{r}'_\perp)\delta(t-t')\delta(z)$, where $\Delta = \Delta^Q/4S_0^2$) and, therefore, can be ignored in comparison to it. This also implies that interfacial *passive* nematic order cannot be facilitated by an active but isotropic interfacial force density, unlike in bulk fluids [3].

That Eq. (24) is stabilising along all directions of the wavevector space when $\zeta\lambda > 0$ and $|\lambda| > 1$ can be shown by reexpressing it in terms of the angle between $\mathbf{q}_\perp$ and $\hat{x}$, $\phi$:

$$\partial_t\theta = \frac{\zeta|q_\perp|}{4\eta}\left[\cos(2\phi)[1-\lambda\cos(2\phi)] - \frac{\lambda}{2}\sin^2(2\phi)\right] + \xi. \tag{26}$$

Let us first consider $\zeta > 0$ and $\lambda > 1$. Then, stability requires that the term within the square brackets to be $< 0$ for all $\phi$. If that is not the case, at least one of its extreme values must be positive. The extreme values of the term in the square brackets, which can rewritten as $[\cos 2\phi - (\lambda/2)(1+\cos^2 2\phi)]$ are at $\phi = (2n+1)\pi/2, n\pi$ or at $\cos 2\phi = 1/\lambda$ (since $|\lambda| > 1$). Then, $[\cos 2\phi - (\lambda/2)(1+\cos^2 2\phi)]|_{\phi=n\pi} = [1-\lambda] < 0$, $[\cos 2\phi - (\lambda/2)(1+\cos^2 2\phi)]|_{\phi=(2n+1)\pi/2} = [-1-\lambda] < 0$ and $[\cos 2\phi - (\lambda/2)(1+\cos^2 2\phi)]|_{\cos\phi=1/\lambda} = [(1/\lambda) - (\lambda/2)\{1+(1/\lambda)^2\}] = 1/(2\lambda) - \lambda/2 < 0$ are all negative when $\lambda > 1$. Similarly, it is easy to see that all the extreme values of the term in the square bracket in (26) are *positive* when $\zeta < 0$ and $\lambda < -1$, which is the condition for stability in that case. In contrast, when $\zeta > 0$ or $\zeta < 0$, and $-1 < \lambda < 1$, the relaxation rate implied by (26) is *negative* i.e., destabilising for some range of $\phi$ as can be easily checked by evaluating it at $\phi = 0$ or $\pi/2$. In contrast to the usual Simha-Ramaswamy instability, however, it is not destabilising either just above or just below $\pi/4$, but away from it.

Eq. (24) can be used to calculate the linear exponents of this model when $\kappa(\mathbf{q}_\perp)$ is positive in all directions of the wavevector space the condition for which was discussed in the main text. For this, I scale $x \to bx$, $y \to b^\mu y$, where $\mu$ is the anisotropy exponent, $t \to b^z t$ where $z$ is the dynamical exponent and $\theta \to b^\chi\theta$ where $\chi$ is the roughness exponent. The values of these linear exponents are fixed by demanding that $\kappa(\mathbf{q}_\perp)$ and the noise strength $\Delta$ remain unchanged upon rescaling for all directions of the wavevector space. Since $\kappa(\mathbf{q}_\perp)$ must remain unchanged along all directions of wavevector space, that immediately implies that $\mu = 1$. Furthermore, since $\kappa(\mathbf{q}_\perp) \sim |q_\perp|$, $z = 1$ as well. The noise strength scales as $\Delta \to \Delta b^{z-\mu-1-2\chi}$ implying that $\chi = -1/2$ since $z = \mu = 1$. As discussed in the main text, the lowest order nonlinearities that are allowed in (24) are of the form $q_\perp(\theta^2)_q$ and the coefficient of this would scale under rescaling as $b^{z-1+\chi} = b^\chi$ which, due the the negativity of $\chi$, is clearly irrelevant. This implies that the long-time, large-scale behaviour predicted by the linear theory is not invalidated by nonlinearities.

The linear exponents (which are also the exact exponents of this model since there is no relevant nonlinearity) could also be obtained by an inspection of the static and dynamic structure factors of angular fluctuations. From (26), these are

$$\langle|\theta(\mathbf{q}_\perp,t)|^2\rangle = \frac{8\eta\Delta}{\zeta|q_\perp|[-2\cos(2\phi)+\lambda\{1+\cos^2(2\phi)\}]}. \tag{27}$$

and, by Fourier transforming (26) in time as well,

$$\langle|\theta(\mathbf{q}_\perp,\omega)|^2\rangle = \frac{128\eta^2\Delta}{64\eta^2\omega^2+\zeta^2 q_\perp^2[M(\phi)]^2}, \tag{28}$$

respectively. Eq. (27) implies that in real space

$$\langle\theta(0,t)\theta(\mathbf{r}_\perp,t)\rangle = \int \frac{d\mathbf{q}_\perp}{4\pi^2} e^{i\mathbf{q}_\perp\cdot\mathbf{r}_\perp}\langle|\theta(\mathbf{q}_\perp,t)|^2\rangle \sim \frac{1}{|\mathbf{r}_\perp|} \tag{29}$$

The decay of angular fluctuations at large scales as $1/|\mathbf{r}_\perp|$ immediately implies that the roughness exponent is $\chi = -1/2$. Furthermore, since Eq. (27) scales the same way along *all* directions of the wavevector space, the anisotropy exponent $\mu = 1$. Finally, balancing $\omega$ against the damping term in (28) yields $\omega \propto q_\perp$ and therefore, the dynamical exponent $z = 1$ within the linearised theory. Note that Eq. (28) still has a zero-frequency pole in the limit of zero wavenumbers i.e., it still describes a Goldstone mode. That is, while the long-range interaction due to a combination of activity and fluid dynamics is sufficiently long-ranged to allow for LRO in two dimensions, it is not long-ranged enough (i.e., it decays too fast) to make the orientational Goldstone mode massive unlike in [24].

As a further direct demonstration of LRO, notice that (27) which, as argued, retains its form even after taking nonlinearities into account, scales as $1/|q_\perp|$ along all directions of the wavevector space. This implies that real space angular fluctuations

$$\begin{aligned}2W = \langle\theta(\mathbf{r}_\perp,t)^2\rangle &= \int \frac{d^2q_\perp}{(2\pi)^2}\frac{8\eta\Delta}{\zeta|q_\perp|[-2\cos(2\phi)+\lambda\{1+\cos^2(2\phi)\}]} \\ &= \int d|q_\perp|\int\frac{d\phi}{\pi^2}\frac{2\eta\Delta}{\zeta[-2\cos(2\phi)+\lambda\{1+\cos^2(2\phi)\}]} \propto \Lambda\Delta\end{aligned} \tag{30}$$

where $\Lambda$ is an upper wavenumber cut-off. $e^{-2W}$ is the Debye-Waller factor which measures the degree to which order-parameter is depressed by fluctuations. Since $W$ doesn't diverge, the Debye-Waller factor is not zero which implies that fluctuations don't depress the order-parameter to 0 even in infinite systems. This clearly and directly demonstrates that the interfacial nematic phase has LRO [18].

As discussed earlier, I have considered scales larger than the Saffman-Delbrück one which controls the crossover between two and three-dimensional momentum conservation. In fact, the equations used till this point essentially take the Saffman-Delbrück scale $\ell sd = 0$. I now briefly discuss how a non-zero, but still small $\ell_{sd}$ modifies the calculation. A non-zero $\ell_{sd}$ will change the spatial scaling of the hydrodynamic kernel from $\sim 1/|q_\perp|$ to $\sim 1/(\ell_{sd}q_\perp^2+|q_\perp|) \approx (1/|q_\perp|)-\ell_s$ when $|q_\perp| \ll 1/\ell_{sd}$. This implies that (26) would have an extra term whose angular character is equivalent to the term in the square brackets in (26) but which scales as $-q_\perp^2\ell_{sd}$. This is a term at $\mathcal{O}(q_\perp^2)$ and therefore competes with the Frank elastic one $-\Gamma_\theta K q_\perp^2\theta$ (since the angular factor in (26) is negative for all $\phi$ when $\zeta\lambda > 0$ and $|\lambda| > 1$, the term arising from the finite Saffman-Delbrück physics is destabilising in this regime and reduces the Frank elasticity anisotropically). Therefore, a finite $\ell_{sd}$ simply renormalises the Frank elasticity (anisotropically). The $\sim q_\perp^2$ term that $\ell_{sd}$ renormalises is irrelevant when the $\sim |q_\perp|$ term is stabilising. When it is destabilising (i.e., when $\zeta\lambda < 0$ or $|\lambda| < 1$), the $\sim q_\perp^2$ term is important for stabilisation at smaller scales and the fastest growing mode beyond the instability depends on the $q_\perp^2$ term.

For completeness, I now calculate the $\mathcal{O}(q_\perp^3)$ term in the angular dynamics arising from passive forces and demonstrate that in the absence of activity, the equal time correlator of angular fluctuations scales as $\sim 1/q_\perp^2$ in all directions, as expected. The contribution of the passive forces to the in-plane velocities is

$$v_x^e = -\int_{-\infty}^{\infty}\frac{dq_z}{2\pi}\frac{iKq_\perp^2}{2\eta q^4}q_y[q^2+\lambda(q_y^2+q_z^2-q_x^2)]\theta = -\frac{iKq_\perp^2}{4\eta|q_\perp|^3}q_y[q_x^2+q_y^2(1+\lambda)]\theta, \tag{31}$$

and

$$v_y^e = \int_{-\infty}^{\infty}\frac{dq_z}{2\pi}\frac{iKq_\perp^2}{2\eta q^4}q_y[q^2-\lambda(q_x^2+q_z^2-q_y^2)]\theta = \frac{iKq_\perp^2}{4\eta|q_\perp|^3}q_x[q_y^2+q_x^2(1-\lambda)]\theta \tag{32}$$

In the equation for angular fluctuations, this then yields the $\mathcal{O}(q_\perp^3)$ term

$$-\frac{[q_x^4(\lambda-1)^2+q_y^4(\lambda+1)^2+2q_x^2q_y^2]}{8\eta|q_\perp|^3}Kq_\perp^2\theta, \tag{33}$$

which is obviously always stabilising. Therefore, in the absence of activity, the angular fluctuations equation would be

$$\partial_t\theta=-\left[\frac{[q_x^4(\lambda-1)^2+q_y^4(\lambda+1)^2+2q_x^2q_y^2]}{8\eta|q_\perp|^3}+\Gamma_\theta\right]Kq_\perp^2\theta+\bar{\xi}+\xi \tag{34}$$

Taking $\Delta=\Gamma_\theta T$ and $\Delta^v=\eta T$, where $T$ is the temperature, as is required for passive systems,

$$\langle\bar{\xi}(\mathbf{q}_\perp,t)\bar{\xi}(\mathbf{q}'_\perp,t)\rangle+\langle\xi(\mathbf{q}_\perp,t)\xi(\mathbf{q}'_\perp,t)\rangle=2T\left[\frac{[q_x^4(\lambda-1)^2+q_y^4(\lambda+1)^2+2q_x^2q_y^2]}{8\eta|q_\perp|^3}+\Gamma_\theta\right]\delta(\mathbf{q}_\perp+\mathbf{q}'_\perp)\delta(t-t') \tag{35}$$

This clearly follows the fluctuation-dissipation relation since the noise correlator is $2T$ times the dissipative coefficient in front of $\delta F/\delta\theta=Kq_\perp^2\theta$ in (34). It is now straightforward to calculate the equal-time correlator for the angular fluctuations which, as expected, is

$$\langle|\theta(\mathbf{q}_\perp,t)|^2\rangle=\frac{T}{Kq_\perp^2} \tag{36}$$

This clearly demonstrates that the long-range order of nematics predicted in the main text is a consequence of activity – a passive nematic at the interface between two fluids only has quasi-long range order and its static correlator can be calculated from the equipartition theorem (as in all equilibrium systems).

### C. Comparison with passive dipolar $X-Y$ models and dynamics of defects

In interfacial active nematics, the momentum-exchange with the bulk fluid leads to an effective long-range interaction that is similar in spirit, and spatially scales the same way as, dipolar interactions in equilibrium $X-Y$ model. I write the angular fluctuations equation (26) (with the additional Frank elastic term) as

$$\partial_t\theta=\frac{\zeta|q_\perp|}{4\eta}\left[\cos(2\phi)[1-\lambda\cos(2\phi)]-\frac{\lambda}{2}\sin^2(2\phi)\right]-\Gamma_\theta Kq_\perp^2\theta+\xi=-\Gamma_\theta\left(\frac{|\zeta|C(\phi)}{4\Gamma_\theta\eta|q_\perp|}+K\right)q_\perp^2\theta+\xi. \tag{37}$$

where $C(\phi)$ is the angular factor in the square brackets times $-\mathrm{sgn}(\zeta)$ and without loss of generality, take $\langle\xi(\mathbf{q}_\perp,t)\xi(\mathbf{q}'_\perp,t')\rangle=2T\Gamma_\theta\delta(\mathbf{q}_\perp+\mathbf{q}'_\perp)\delta(t+t')$ for some $T$. Since I am considering the dynamics when the ordered phase is linearly stable, $C(\phi)>0$ for all $\phi$. It is then clear that the dynamics of $\theta$ can be considered to be governed by an effective free-energy of the form

$$F_{\text{eff}}[\theta]=\frac{1}{2}\int d|q_\perp|\int d\phi\left[\frac{|\zeta|C(\phi)}{4\Gamma_\theta\eta}\frac{1}{|q_\perp|}+K\right]q_\perp^2|\theta|^2 \tag{38}$$

Importantly, the first term in the square bracket has the same spatial character as the dipolar energy in a two-dimensional $X-Y$ model with dipolar interactions [19–21] which, in real space has the free energy density

$$F_{\text{dip}}=\int_{\mathbf{r}_\perp}\int_{\mathbf{r}'_\perp}\frac{\partial_\alpha\theta(\mathbf{r}_\perp)\partial'_\beta\theta(\mathbf{r}'_\perp)}{|\mathbf{r}_\perp-\mathbf{r}'_\perp|} \tag{39}$$

which also displays long-range order in two dimensions (in fact, it displays long-range order for $d>1$). This further supports the prediction of long-range active nematic order at an immersed interface. However, the angular factor $C(\phi)$ associated with the long-range hydrodynamic interaction in this system is distinct from the angular factor in a dipolar $X-Y$ magnet; in particular, in interfacial nematics, $C(\phi)$ is strictly greater than 0 for all $\phi$ when $\zeta\lambda>0$ and $|\lambda|>1$ while the angular factor associated with dipolar interactions in a dipolar $X-Y$ model vanishes along the ordering direction. This distinction significantly modifies the physics of the ordered phase; the exponents of the ordered phase that I calculate for the interfacial active nematics are different from those for the dipolar $X-Y$ model. The linear exponents for the dipolar $X-Y$ model can, in fact be calculated just from the knowledge that the dipolar interaction scales spatially as $1/|q_\perp|$ and its angular part vanishes for $\phi=0$. They are: the dynamical exponent $z=2$, the anisotropy exponent $\mu=3/2$ and the roughness exponent $\chi=-1/4$. However, these exponents will be

modified for active extensions of the passive dipolar $X - Y$ model relevant, for instance, for polar active particles on a substrate interacting via long-range dipolar interactions. The value of the roughness exponent for the interfacial active nematic that I calculate, $\chi = -1/2$, shows that it has an even greater degree of order, i.e. its long wavelength angular fluctuations are even smaller, than the passive dipolar $X - Y$ model. This distinction will however not have a significant impact on the interaction of defects which I now discuss.

In the main text, I noted that the long-range interaction due to hydrodynamics also affects the dynamics of defects in the nematic fluid at the interface. I discuss this in slightly greater detail here. The defect interactions are governed by the same process that leads to the relaxation of the angular fluctuations (see the supplement of [25]). I can therefore use (38) to heuristically obtain the scaling of the effective defect interactions, ignoring the motility of $+1/2$ defects. This is in direct analogy with the argument presented in [20] for vortex interactions in passive dipolar $X - Y$ model. The singular part of the angle field due to a defect at the origin with charge $s$ can be written as

$$\bar{\theta}(|r_\perp|, \phi') = 2\pi s \int_{|q_\perp|,\phi} \frac{e^{i|q_\perp||r_\perp|\cos(\phi-\phi')}}{q_\perp^2} \tag{40}$$

and, from this, the defect interaction energy between two defects (which can be easily generalised to arbitrary number of defects), with charges $s_1$ and $s_2$ and positions 0 and $|r_\perp|(\cos\phi', \sin\phi')$ can be obtained as

$$F_{def} = \pi^2 s_1 s_2 \int_{|q_\perp|,\phi} e^{-i|q_\perp||r_\perp|\cos(\phi-\phi')} \left[\frac{K}{q_\perp^2} + \frac{|\zeta|C(\phi)}{4\Gamma_\theta\eta}\frac{1}{|q_\perp|}\right]. \tag{41}$$

As is well-known, the infrared divergences cancel for a charge-neutral system finally yielding a defect interaction energy (for one of the defects at the origin) which, when written in real space has the form

$$F_{int} = -s_1 s_2 \left[\frac{\pi K}{2}\ln\left(\frac{|r_\perp|}{a}\right) + \frac{\zeta}{\Gamma_\theta\eta}\alpha|r_\perp|\right] \tag{42}$$

where $a$ is the size of the defect core and $\alpha > 0$ is a positive constant whose determination requires a detailed calculation far beyond the scope of this heuristic argument. The interaction energy scaling as $|r_\perp|$ is stronger than the usual logarithmic potential that binds defects in passive systems with short-range interactions and is equivalent to the potential between vortices in dipolar $X - Y$ models. In passive dipolar $X - Y$ models, this immediately implies that defects are bound in the low temperature ordered phase. The situation is more complicated here because of two aspects of defect dynamics in active systems both of which I disregarded here: i. Self-propulsion of $+1/2$ defects. Within a one-dimensional approximation, this leads to an effective *repulsive* potential between oppositely charged defects that scales as $|r_\perp|$ and should compete against the attractive potential $\propto \zeta$ here. This repulsive potential also depends linearly on $\zeta$ and therefore whether defects remain bound in the ordered phase would require a detailed calculation of the coefficients of the defect motility and attractive interaction in this case. While this picture is essentially correct at *low* noise strengths, [25] demonstrates that at intermediate noise strengths fluctuations isotropise the direction of motion of the $+1/2$ defects, weakening the effect of motility (however, fluctuations don't qualitatively modify the *attractive* interaction $\propto \zeta$ in (42)). Therefore, at least at intermediate noise strengths, the defects should remain strongly bound making the long-range ordered phase described here possible. The examination of whether there is an active defect-driven transition from the nematic to the isotropic phase at *low* noise is significantly more complicated and will be dealt with elsewhere. ii. In addition to this, defects in an active system are also dragged by the velocity field generated by other defects [25] which leads to non-mutual interaction between defects [26–28]. A consideration of these complexities will be discussed elsewhere. Notwithstanding these caveats, the present heuristic calculation suggests that the long-range ordered nematic state discussed here should be observable in experiments and will not be inevitably destroyed due to the unbinding of defects.

## II. NUMBER CONSERVED ACTIVE NEMATICS AT THE INTERFACE BETWEEN TWO FLUIDS

Till now, I have tacitly considered a system in which the number of active units is not conserved. If I consider a system in which the concentration of active units is a conserved quantity, with a mean concentration $c_0$, the concentration field has a linearised continuity equation given by

$$\partial_t c = -c_0 \nabla_\perp \cdot \mathbf{v} + \zeta_Q \partial_x \partial_y \theta + D\nabla_\perp^2 c + \xi_c, \tag{43}$$

where $\langle \xi_c(\mathbf{r}_\perp, t)\xi_c(\mathbf{r}'_\perp, t')\rangle = -2\Delta^c \nabla_\perp^2 \delta(\mathbf{x} - \mathbf{x}')\delta(t - t')$. while the angle field equation remains unchanged:

$$\partial_t \theta = \Omega_{xy} - \lambda A_{xy} + \Gamma K \nabla_\perp^2 \theta + \xi \tag{44}$$

To leading order the linearised constitutive equation for the Stokesian velocity field is

$$\eta\nabla^2 V_x = \partial_x \Pi + \partial_x \frac{\delta F}{\delta c}\delta(z) + \zeta(c_0)\partial_y\theta\delta(z) + \zeta_1\partial_x c\delta(z) + \zeta_c\partial_x c\delta(z) + \xi_x^v \tag{45}$$

$$\eta\nabla^2 V_y = \partial_y \Pi + \partial_y \frac{\delta F}{\delta c}\delta(z) + \zeta(c_0)\partial_x\theta\delta(z) - \zeta_1\partial_y c\delta(z) + \zeta_c\partial_y c\delta(z) + \xi_y^v \tag{46}$$

$$\eta\nabla^2 V_z = \partial_z \Pi + \xi_z^v \tag{47}$$

where the free energy $F = \int d\mathbf{r}_\perp[A(\delta c)^2 + (K/2)(\nabla_\perp\theta)^2 + K_c\delta c\partial_x\partial_y\theta]$ [4, 5], with $\delta c = c - c_0$, $\zeta_1 \equiv (1/2)\partial_c\zeta|_{c=c_0}$ and the term with the coefficient $\zeta_c$ arises from an active isotropic stress. Calculating the in-plane velocity field at $z = 0$ as earlier and defining $A_r = A + \zeta_c$, I then get the coupled equations for the angle and concentration fields to $\mathcal{O}(q_\perp)$:

$$\partial_t\theta = -\frac{\zeta}{4\eta}\frac{q_x^4(\lambda-1) + q_y^4(\lambda+1)}{|q_\perp|^3}\theta - \frac{q_xq_y[q_x^2\{A_r\lambda - (\lambda-2)\zeta_1\} + q_y^2\{A_r\lambda + (\lambda+2)\zeta_1\}]}{4\eta|q_\perp|^3}\delta c + \xi, \tag{48}$$

and

$$\partial_t\delta c = -\frac{\zeta c_0 q_x q_y}{2\eta|q_\perp|}\theta - \frac{c_0q_x^2(A_r+\zeta_1) + c_0q_y^2(A_r-\zeta_1)}{4\eta|q_\perp|}\delta c + \bar{\xi}_c + \xi_c \tag{49}$$

where $\delta c = c - c_0$, $\bar{\xi}_c$ is the noise in the concentration equation that appears due to the coupling to the velocity field via the $-c_0\nabla_\perp\cdot\mathbf{v}$ coupling and, in Fourier space, has the correlation

$$\langle\bar{\xi}_c(\mathbf{q}_\perp,t)\bar{\xi}_c(\mathbf{q}'_\perp,t')\rangle = \frac{2c_0^2\Delta^v|q_\perp|}{4\eta^2}\delta(\mathbf{q}_\perp + \mathbf{q}'_\perp)\delta(t-t'). \tag{50}$$

All terms in (49) are $\mathcal{O}(q_\perp)$ and arise from the $\nabla_\perp\cdot\mathbf{v}$ term which is non-zero since there is no constraint of *in-plane* incompressibility (only bulk incompressibility). The other terms in (43) are $\mathcal{O}(q_\perp^2$ and, therefore, have been ignored in writing (43). Furthermore, the correlator of the noise $\xi_c$ vanishes at large scales as $\sim q_\perp^2$ and it is therefore subdominant to $\bar{\xi}_c$ and will be ignored. The eigenfrequencies of the coupled concentration and angular dynamics, from (48) and (49) are

$$\omega_\pm = -\frac{i|q_\perp|}{8\eta}\Bigg[(A_r + \zeta_1\cos 2\phi)c_0 - \zeta\cos 2\phi(1-\lambda\cos 2\phi) + \frac{\zeta\lambda}{2}\sin^2 2\phi \pm\sqrt{\left\{(A_r + \zeta_1\cos 2\phi)c_0 - \zeta\cos 2\phi(1-\lambda\cos 2\phi) + \frac{\zeta\lambda}{2}\sin^2 2\phi\right\}^2 + 4c_0\zeta\{\zeta_1 + A_r\cos 2\phi\}(1-\lambda\cos 2\phi)}\Bigg] \tag{51}$$

At least one of the eigenvalues $\omega_\pm$ has a positive imaginary part for some $\phi$, implying that the homogeneous nematic phase is destabilised, except for special values of the parameters: $A_r > |\zeta_1|$, $\lambda = -A_r/\zeta_1$ and $\zeta\zeta_1 < 0$. In this case, the eigenfrequencies become

$$\omega_\pm = -\frac{i|q_\perp|}{8\eta}\Bigg[(c_0\zeta_1 - \zeta)\cos 2\phi + c_0A_r - \frac{A_r\zeta}{2\zeta_1}(1+\cos^2 2\phi) \pm\sqrt{\left\{(\zeta - c_0\zeta_1)\cos 2\phi - c_0A_r + \frac{A_r\zeta}{2\zeta_1}(1+\cos^2 2\phi)\right\}^2 + 4\frac{c_0\zeta}{\zeta_1}\{\zeta_1 + A_r\cos 2\phi\}^2}\Bigg] \tag{52}$$

It is clear that when $A_r > |\zeta_1|$ and $\zeta\zeta_1 < 0$, the term inside the square bracket and outside the square root is always positive while the magnitude of the term inside the square root is always smaller than the term outside the square root (since $\zeta\zeta_1 < 0$). Therefore, both $\omega_\pm$ has a negative imaginary part for all $\phi$ in this case. However, $\omega_-$ is 0 for some specific $\phi$. In these directions, the eigenfrequency has to be extended to $\mathcal{O}(q_\perp^2)$. Since the $\mathcal{O}(q_\perp^2)$ part of the eigenfrequency is only important along these particular directions of the wavevector space, I simply add an isotropic $\sim q_\perp^2$ term to the relaxation rate and define $\kappa_+ = i\omega_+$ and $\kappa_- = i\omega_- + \bar{K}q_\perp^2$. Then, the dynamic structure factor of concentration fluctuations is

$$\langle|\delta c(\mathbf{q}_\perp,\omega|^2\rangle = \frac{2\zeta^2c_0^2\sin^2 2\phi\Delta|q_\perp|^2}{16\eta^2(\omega^2+\kappa_+^2)(\omega^2+\kappa_-^2)} \tag{53}$$

which yields the static structure factor

$$\langle|\delta c(\mathbf{q}_\perp,t|^2\rangle = \frac{\zeta^2 c_0^2 \sin^2 2\phi \Delta |q_\perp|^2}{16\eta^2(\kappa_+^2\kappa_- + \kappa_-^2\kappa_+)} \tag{54}$$

Since the the numerator vanishes at $n\pi/2$, where $n$ is an integer, and $i\omega_-$ vanishes at a $\phi$ depending on the ratio of $A_r/\zeta_1$ and not at $\phi = n\pi/2$, (54) is clearly the most divergent when $i\omega_-$ vanishes. Defining $\phi_0$ as the points at which $i\omega_-$ vanishes, I expand $\kappa_- = A_1(\delta\phi)^2|q_\perp| + \bar{K}q_\perp^2$ around these points where $\delta\phi = \phi - \phi_0$ and $A_1$ is a constant whose value depends on $\zeta$, $A_r$ and $\zeta_1$. The real space concentration fluctuations scale as

$$\langle|\delta c(\mathbf{r}_\perp,t|^2\rangle = \int \frac{dq_x dq_y}{(2\pi)^2}\langle|\delta c(\mathbf{q}_\perp,t|^2\rangle \approx S\int |q_\perp| d|q_\perp| \int_{-\infty}^{\infty} d\delta\phi \frac{1}{(\delta\phi)^2|q_\perp| + B^2|q_\perp|^2} \tag{55}$$

where $S$ and $B$ are constants. I have extended the range of the angular integral to $\pm\infty$ since it is dominated by $\delta\phi \ll 1$. Evaluating the angular integral,

$$\int_{-\infty}^{\infty} d\delta\phi \frac{1}{(\delta\phi)^2|q_\perp| + B^2|q_\perp|^2} = \frac{\pi}{B|q_\perp|^{3/2}} \tag{56}$$

This implies that the static structure factor of concentration fluctuations (54) diverges as $\sim 1/|q_\perp|^{3/2}$. This divergence implies that the R.M.S. number fluctuations in $\sqrt{\langle\delta N\rangle^2}$ in a region containing on average $\langle N\rangle$ particles scales as $\langle N\rangle^{7/8}$ instead of $\sim \langle N\rangle^{1/2}$ as in all equilibrium systems or as $\langle N\rangle$ as in stable active nematics on a substrate. However, I emphasise that this is an extreme special case which requires tuning the values of various coefficients such that $A_r > |\zeta_1|$, $\lambda = -A_r/\zeta_1$ and $\zeta\zeta_1 < 0$. Therefore, this is unlikely to be observed in experiments. For all other values of the parameters the homogeneous nematic phase is destabilised. As discussed in the main text, this is most clearly seen for very large $A_r$ in which case the eigenfrequencies become

$$\omega_+ = -\frac{ic_0}{4\eta}A_r|q_\perp| \tag{57}$$

and

$$\omega_- = \frac{i\zeta}{4\eta}|q_\perp|\cos 2\phi(1-\lambda\cos 2\phi). \tag{58}$$

The former eigenvalue, $\omega_+$ signals an infinitely fast relaxation of the concentration fluctuations as $A_r \to \infty$ while the latter eigenvalue $\omega_-$ implies a dynamics that is equivalent to an incompressible active nematic layer in three-dimensional fluid which is generically unstable and has the same angular character as the Simha-Ramaswamy instability [6]. This is expected: A large $A_r$ implies that the dynamics is extremely sensitive to departures of $c$ from the mean concentration of particles $c_0$, enforcing an effective two-dimensional incompressibility constraint in this limit. This is the sense in which the two-dimensional incompressibility constraint in [8–10] should be viewed.

I now discuss the instability implied by (51) in greater detail, in particular focussing on the similarity and distinction of this with the usual Simha-Ramaswamy instability, which I showed is obtained in the limit of large $A_r$. For this, I consider (51) in the special case in which $\zeta_1 = 0$, which highlights the distinction. In this case, the eigenfrequencies become

$$\omega_\pm = -\frac{i|q_\perp|}{32\eta}\left[\{4A_r c_0 + 2\zeta\lambda(1+\cos^2 2\phi) - 4\zeta\cos 2\phi)\} \pm \sqrt{64A_r c_0\zeta(1-\lambda\cos 2\phi) + \{4A_r c_0 + 2\zeta\lambda(1+\cos^2 2\phi) - 4\zeta\cos 2\phi)\}^2}\right] \tag{59}$$

It is clear that when $A_r = 0$, $\omega_-$ vanishes to $\mathcal{O}(q_\perp)$ (i.e., $\omega_- \sim q_\perp^2$) while the other eigenfrequency has the value

$$\omega_+(A_r = 0) = \frac{i\zeta|q_\perp|}{8\eta}[2\cos 2\phi - \lambda(1+\cos^2 2\phi)] = \frac{i\zeta|q_\perp|}{4\eta}\left[\cos 2\phi(1-\lambda\cos 2\phi) - \frac{\lambda}{2}\sin^2 2\phi\right], \tag{60}$$

which is exactly equivalent to the eigenfrequency for a film without a conserved, two-dimensional concentration field at the interface. The reason that to leading order $\omega_+$ for a film with a conserved number of nematogens reduces to one in which the nematogen number is not conserved, in the limit of vanishing effective compressibility $A_r \to 0$ has to do with the structure of the equations of motion. First, notice that in this limit, the equation of motion for the velocity field has no contribution from the concentration field at $\mathcal{O}(q_\perp)$. Therefore, the equation for angular fluctuations is decoupled from that of the concentration fluctuations at $\mathcal{O}(q_\perp)$. Furthermore, since the velocity field is independent

of the concentration fluctuations to $\mathcal{O}(q_\perp)$, the eigenvalue corresponding to the concentration fluctuations is simply $\omega_- = -iDq_\perp^2$ to leading order in wavenumbers (a term $\gamma_Q \partial_x \partial_y \delta c$ is potentially present in the angular dynamics at second order in wavenumbers, but even with the inclusion of this the eigenvalue remains stable for small enough $\gamma_Q$).

I will now examine $\omega_\pm$ for both large and small $A_r$. First, at large $A_r$, the eigenfrequency which has a non-zero negative imaginary value for $A_r = 0$ remains stabilising and its magnitude diverges with $A_r$:

$$\omega_+ \sim -\frac{ic_0|q_\perp|}{4\eta} A_r \tag{61}$$

implying an infinitely fast relaxation of the concentration field, in the $A_r \to \infty$ limit, which is the characteristic of an incompressible system. The the other eigenfrequency, the one that vanishes when $A_r = 0$, assumes a value that is independent of $A_r$:

$$\omega_- \sim \frac{i\zeta|q_\perp|}{4\eta} \cos 2\phi (1 - \lambda \cos 2\phi). \tag{62}$$

This is the eigenfrequency characteristic of the Simha-Ramaswamy instability which appears here in the $A_r \to \infty$ limit. As is well known, this implies an instability of the uniaxial phase irrespective of parameter values. More precisely, an extensile suspension $\zeta > 0$ is unstable to bend fluctuations with $\phi \lesssim \pi/4$ while a contractile active fluid is unstable to splay fluctuations at $\phi \gtrsim \pi/4$ as $A_r \to \infty$. Next, we look at the behaviour of the eigenfrequencies at small $A_r$ which turns out to be more interesting. As discussed above, the imaginary part of $\omega_+$ goes to a finite negative value at $A_r = 0$ for all $\phi$ (when $\zeta\lambda > 0$ and $\lambda > 1$; the maximum value of $\mathrm{Im}[\omega_+]$ is otherwise positive at $A_r = 0$). The other eigenfrequency, which vanishes at $A_r = 0$, and goes to the usual Simha-Ramaswamy result (62) at large $A_r$, *increases linearly* with $A_r$ at small $A_r$:

$$\lim_{A_r \to 0} \omega_- = \frac{iA_r c_0 |q_\perp|}{8\eta} \left[ -1 - \frac{\lambda - 4\cos 2\phi + 3\lambda \cos 4\phi}{-4\cos 2\phi + \lambda(3 + \cos 4\phi)} \right]. \tag{63}$$

Importantly, this eigenfrequency becomes *independent* of $\zeta$, and therefore, of its sign, at small $A_r$ (i.e., when $\zeta\lambda \gg A_r c_0$. Of course, $\omega_-$ vanishes when $\zeta = 0$). This feature does not depend on $\zeta_1$ being 0. The R.H.S. of (63) vanishes generically for $\phi = \pi/4$ implying that it is unstable even at small $A_r$ either for $\phi \gtrsim \pi/4$ or for $\phi \lesssim \pi/4$ depending only on the value of $\lambda$. This is clearly seen by expanding (63) around $\phi = \pi/4$ for small $A_r$:

$$\lim_{A_r \to 0} \omega_-(\phi \approx \pi/4) \approx -\frac{iA_r c_0 |q_\perp|}{\eta\lambda} \left[ \phi - \frac{\pi}{4} \right]. \tag{64}$$

This eigenfrequency signifies an instability whose growth rate grows with $A_r$ at small $A_r$. Expanding $\omega_-$ (59) about $\pi/4$, I then find that it doesn't depend on $A_r$ beyond a critical value $\propto \zeta\lambda$, as the concentration is increased.

$$\omega_-(\phi \approx \pi/4) \approx -\frac{iA_r c_0 |q_\perp| \zeta}{2A_r c_0 \eta + \zeta\eta\lambda} \left[ \phi - \frac{\pi}{4} \right]. \tag{65}$$

This result significantly extends the original Simha-Ramaswamy instability and demonstrates that uniaxial active ordering at an interface, which is generically compressible, is always unstable if the number of orientable active filaments *at the interface* is conserved but, crucially, the character of the instability changes with the effective compressibility $1/A_r$ of the conserved orientable species controlled by the density.

The above discussion focussed on the case in which an anisotropic, active, concentration-dependent force vanishes i.e., $\zeta_1 = 0$. That is because I wanted to uncover the effect of going from an effective compressible layer to an effectively incompressible one, upon changing the global (conserved), two-dimensional density field at the interface which leads to a change in the effective two-dimensional compressibility at the interface. The force $\propto \zeta_1$ also modifies the character and the angular character of the instability but cannot eliminate it.

This discussion of the modification of the character of the active instability as the compressibility of the conserved nematogenic species at the interface is increased, achievable, for instance, by decreasing the global density, has an important experimental consequence. It is generally assumed that the characteristic wavelength of the active instability at an interface scales as $1/\zeta$. However, I showed that at small $A_r$ i.e., for a low density of active units, the instability growth rate becomes independent of $\zeta$. The fastest growing wavevector may be calculated by retaining the $\mathcal{O}(q_\perp^2)$ stabilising terms. While these terms will also generically depend on activity, they do not vanish in the limit of vanishing activity [8]. Thus, at least for sufficiently small activity, as the density of the conserved orientable active particles at the interface is reduced, the fastest growing mode should become independent of activity [8]. In experiments on motor-microtubule filaments at a fluid-fluid interface, the number of the microtubule bundles at the interface is essentially conserved and activity is generally controlled by the concentration of kinesin motors. Therefore, this theory implies that as the microtubule concentration is reduced, the fastest growing mode should become independent of kinesin concentration. This prediction may be checked in existing experimental setups for experiments on motor-microtubule films at two-fluid interfaces.

## III. NUMBER CONSERVED POLAR PHASE AT THE INTERFACE BETWEEN TWO FLUIDS

In this section, I describe an interfacial polar active phase. The polarisation field is described by an in-plane polar vector $\mathbf{p}$ which is taken to be ordered along the $\hat{x}$ direction $\mathbf{p} = p_0(\cos\theta, \sin\theta)$. The free energy, in terms of the concentration field and the soft angle field $\theta$ is now $F = \int d\mathbf{r}_\perp[A(\delta c)^2 + (K/2)(\nabla_\perp\theta)^2 + \gamma\delta c\partial_y\theta]$. Even at the leading order, two new active effects need to be considered in a polar fluid: i. self-advection of the polarisation field via a term $v_p(c)\mathbf{p}\cdot\nabla\mathbf{p}$ and ii. a concentration current $v_c(c)\mathbf{p}$ due to motility [11–14]. This implies that the linearised equations for the concentration and angular fluctuations are

$$\partial_t\delta c = -c_0\nabla_\perp\cdot\mathbf{v} - \bar{v}_c p_0\partial_x c - v_c p_0\partial_y\theta + D\nabla_\perp^2\delta c + \xi_c \tag{66}$$

where $\bar{v}_c = \partial_c v_c|_{c=c_0}$ and

$$\partial_t\theta = -v_p p_0\partial_x\theta + \Omega_{xy} - \lambda A_{xy} - \Gamma_\theta\frac{\delta F}{\delta\theta} + \xi \tag{67}$$

The active stress for the polar fluid is $\bar{\zeta}[\mathbf{pp} - (1/2)p^2\mathbf{I}]$, and defining $\zeta = \bar{\zeta}p_0^2$, the linear equation for the velocity field is

$$\eta\nabla^2 V_x = \partial_x\Pi + \partial_x\frac{\delta F}{\delta c}\delta(z) + \zeta\partial_y\theta\delta(z) + \zeta_1\partial_x c\delta(z) + \zeta_c\partial_x c\delta(z) + \xi_x^v \tag{68}$$

$$\eta\nabla^2 V_y = \partial_y\Pi + \partial_y\frac{\delta F}{\delta c}\delta(z) + \zeta\partial_x\theta\delta(z) - \zeta_1\partial_y c\delta(z) + \zeta_c\partial_y c\delta(z) + \xi_y^v \tag{69}$$

$$\eta\nabla^2 V_z = \partial_z\Pi + \xi_z^v \tag{70}$$

As in the earlier sections, I eliminate the velocity field to obtain the coupled equations of motion for the concentration and the angle fields which, upon again defining $A_r = A + \zeta_c$, reads

$$\partial_t\theta = -\frac{\zeta}{4\eta}\frac{q_x^4(\lambda-1) + q_y^4(\lambda+1)}{|q_\perp|^3}\theta - \frac{q_x q_y[q_x^2\{A_r\lambda - (\lambda-2)\zeta_1\} + q_y^2\{A_r\lambda + (\lambda+2)\zeta_1\}]}{4\eta|q_\perp|^3}\delta c - i\Gamma_\theta\gamma q_y\delta c - iv_p p_0 q_x\theta + \xi, \tag{71}$$

and

$$\partial_t\delta c = -\frac{\zeta c_0 q_x q_y}{2\eta|q_\perp|}\theta - \frac{c_0 q_x^2(A_r+\zeta_1) + c_0 q_y^2(A_r - \zeta_1)}{4\eta|q_\perp|}\delta c - i\bar{v}_c p_0 q_x\delta c - iv_c p_0 q_y\theta + \bar{\xi}_c \tag{72}$$

The general eigenfrequencies implied by (71) and (72) are too involved to present in full and not very illuminating. Instead, I look at some special cases. First, I look at the case when the active system is effectively incompressible in *two-dimensions* for very large $A_r$ (much larger than $\zeta$, $\zeta_1$). In this case, the eigenvalues are

$$\omega_+ = \left[p_0\bar{v}_c\cos\phi + \frac{v_c\lambda}{c_0}\sin^2\phi\cos\phi - \frac{ic_0}{4\eta}(A+\zeta_c)\right]|q_\perp| \tag{73}$$

and

$$\omega_- = \left[p_0 v_p\cos\phi - \frac{v_c\lambda}{c_0}\sin^2\phi\cos\phi + \frac{i\zeta}{4\eta}\cos 2\phi(1-\lambda\cos 2\phi)\right]|q_\perp|. \tag{74}$$

As expected, $\mathrm{Im}[\omega_-] > 0$ for $\phi \lesssim \pi/4$ when $\zeta > 0$ and for $\phi \gtrsim \pi/4$ for $\zeta < 0$ leading to the Simha-Ramaswamy instability of the homogeneous polar phase. However, unlike the homogeneous nematic state (which is stable only when a specific relation among parameters is satisfied), the polar state is stable for a range of parameters. I demonstrate this in the limit of large $v_p$ or large $\bar{v}_c$. In both limits, the eigenfrequencies are

$$\omega_+ = \left[\bar{v}_c p_0\cos\phi - i\frac{c_0}{4\eta}(A_r + \zeta_1\cos 2\phi)\right]|q_\perp| \tag{75}$$

and

$$\omega_- = \left[ v_p p_0 \cos\phi + \frac{i\zeta}{4\eta}\left\{ \cos 2\phi(1-\lambda\cos 2\phi) - \frac{\lambda}{2}\sin^2 2\phi \right\}\right] |q_\perp| \tag{76}$$

when $\phi \neq \pi/2$ (this holds for $\phi \in [0, \pi/2)$ in the limit of diverging $v_p$ or $\bar{v}_c$, but closer one gets to $\phi = \pi/2$, the larger $v_p$ or $\bar{v}_c$ must be for these to hold). For $\zeta\lambda > 0$, $|\lambda| > 1$ and $A_r > \zeta_1$, they describe stable modes whose propagative part and damping are both $\mathcal{O}(q_\perp)$. This implies that if the eigenfrequencies fluctuations along $\phi = \pi/2$ are also stabilising, the homogeneous polar state is stable for large $v_p$ or large $\bar{v}_c$. Explicitly calculating the eigenfrequencies for fluctuations along $\phi = \pi/2$

$$\omega_\pm(\phi = \pi/2) = -\frac{i|q_\perp|}{8\eta}\left[(A_r - \zeta_1)c_0 + \zeta(1+\lambda) \pm \sqrt{\{\zeta(1+\lambda) - (A_r-\zeta_1)c_0\}^2 - 64 p_0 v_c \gamma\eta^2}\right] \tag{77}$$

I find that neither of them is generically destabilising i.e., the imaginary part of either of these is not generically positive; in particular, it is stabilising when $\gamma v_c > 0$. This implies that LRO interfacial homogeneous polar phases are stable in some regime of the parameter space.

To understand the "outrunning" of the instability due to the motility better, I now write the eigenfrequencies corresponding to (71) and (72) in the simple case in which $\bar{v}_c = 0$, $v_c = 0$, $\gamma = 0$ and $\zeta_1 = 0$ (note that the stable regime was obtained in limit in which either $\bar{v}_c$ or $v_p$ was large; in this simplifying case, I will focus on the latter). For this, I define

$$\mathcal{M}(\phi) = -A_r c_0 - \frac{\zeta\lambda}{2}(1+\cos^2 2\phi) - 4ip_0 v_p \eta\cos\phi + \zeta\cos 2\phi \tag{78}$$

and get

$$\omega_\pm = \frac{|q_\perp|}{8\eta}\left[\mathcal{M}(\phi) \pm \sqrt{\mathcal{M}(\phi)^2 - A_r c_0\{4ip_0 v_p\eta\cos\phi - \zeta\cos 2\phi(1-\lambda\cos 2\phi)\}}\right]. \tag{79}$$

It is clear that for large $v_p$ ($v_p\eta \gg A_r c_0, \zeta$), the term $\propto v_p^2$ appearing from $\mathcal{M}(\phi)^2$ dominates inside the square root when $\cos\phi \neq= 0$. A simple expansion then yields the following eigenfrequencies for large $v_p$:

$$\omega_+ = -i\frac{c_0}{4\eta}A_r|q_\perp| + \mathcal{O}\left(\frac{1}{v_p}\right) \tag{80}$$

and

$$\omega_- = \left[v_p p_0\cos\phi + \frac{i\zeta}{4\eta}\left\{\cos 2\phi(1-\lambda\cos 2\phi) - \frac{\lambda}{2}\sin^2 2\phi\right\}\right]|q_\perp| + \mathcal{O}\left(\frac{1}{v_p}\right). \tag{81}$$

This outrunning of the instability due to the motility is only possible since the growth rate of the nematic instability is itself $\sim q_\perp$ due to the momentum-exchange of the layer with the bulk fluid. Such a possibility would not have existed in a Stokesian, bulk nematic fluid where the growth rate would be wavevector-independent.

I now calculate the number fluctuations for a stable interfacial polar flock. For this, writing $-\mathrm{Im}[\omega_\pm] = \kappa_\pm$ and $\mathrm{Re}[\omega_\pm] = c_\pm$, I calculate the dynamic structure factor of concentration fluctuations as

$$\langle|\delta c(\mathbf{q}_\perp,\omega|^2\rangle = \frac{2(\zeta^2 c_0^2\sin^2 2\phi + 16\eta^2 v_c^2 p_0^2 \sin^2\phi)\Delta|q_\perp|^2}{16\eta^2\{(\omega-c_+)^2+\kappa_+^2\}\{(\omega-c_-)^2+\kappa_-^2\}} \tag{82}$$

where both $c_\pm$ and $\kappa_\pm$ are $\mathcal{O}(|q_\perp|)$. The static structure factor is

$$\langle|\delta c(\mathbf{q}_\perp,t|^2\rangle = \frac{(\zeta^2 c_0^2\sin^2 2\phi + 16\eta^2 v_c^2 p_0^2\sin^2\phi)\Delta|q_\perp|^2(\kappa_+ + \kappa_-)}{16\eta^2\kappa_+\kappa_-\{(c_+-c_-)^2+(\kappa_++\kappa_-)^2\}} \propto \frac{1}{|q_\perp|} \tag{83}$$

The $1/|q_\perp|$ divergence of the static structure factor of concentration fluctuations implies that the R.M.S. number fluctuations $\sqrt{\langle\delta N^2\rangle}$ in a region with $\langle N\rangle$ particles on average scales as $\langle N\rangle^{3/4}$, instead of as $\langle N\rangle^{1/2}$ as it would in all equilibrium systems, and thus violates the law of large numbers.

Moreover, the linearised exponents for the concentration fluctuation discussed for the apolar model remains the same in this case as well, i.e., $z = 1$, $\mu = 1$ and $\chi = -1/2$. Defining the roughness exponent for the concentration fluctuations as $\delta c \to b^{\chi_c}\delta c$, it is clear from (83) that $\chi_c = -1/2$ as well within the linear theory. Since the lowest

order nonlinearities, arising either from the flow couplings or advection or motility in either equation must scale as $q_\perp(\theta^2)_{q_\perp}$, $q_\perp(\delta c^2)_{q_\perp}$ or $q_\perp(\delta c\theta)_{q_\perp}$, all of them are irrelevant since $\mu = z = 1$ and $\chi = \chi_c < 0$. Therefore, the linear theory discussed here remains valid even upon the inclusion of nonlinearities.

Polar active systems are also distinguished from their nematic counterparts by a polar active force $\mathbf{f}_p = \zeta_p(\nabla_\perp^2\mathbf{p} + \nabla_\perp\nabla_\perp\cdot\mathbf{p})\delta(z)$ which I had ignored till now since it appears at a higher order in gradients compared to the active force $\propto \zeta$. I now demonstrate that the inclusion of this does not modify any physics discussed here. The in-plane velocities due to this active force are

$$v_x^p = \int_{-\infty}^{\infty}\frac{dq_z}{2\pi}\frac{\zeta_p}{\eta q^4}q_y q_x(q_x^2 - q_z^2)\theta = -\frac{\zeta_p}{4\eta|q_\perp|^3}q_y^3 q_x\theta, \tag{84}$$

and

$$v_y^p = -\int_{-\infty}^{\infty}\frac{dq_z}{2\pi}\frac{\zeta_p}{\eta q^4}(q_x^4 + q_z^2 q_\perp^2)\theta = -\frac{\zeta_p}{4\eta|q_\perp|^3}(q_x^4 + q_\perp^4)\theta. \tag{85}$$

In the equation for angular fluctuations, this yields an extra term

$$\partial_t\theta = \mathcal{O}(q_\perp) + \frac{i\zeta_p q_x\{q_x^2 q_\perp^2(\lambda - 1) + \lambda q_y^4\}}{4\eta|q_\perp|^3}\theta + .... \tag{86}$$

where I have only highlighted the part coming from the polar active stress and suppressed all other pieces including the one coming from Frank elasticity at $\mathcal{O}(q_\perp^2)$, which is $-\Gamma_\theta K q_\perp^2\theta$. As could be seen from power counting, this is a $\mathcal{O}(q_\perp^2)$ *propagative* term. Similarly, it also yields a $\mathcal{O}(q_\perp^2)$ term $\partial_t c = \mathcal{O}(q_\perp) + [(1/4\eta|q_\perp|)i\zeta_p c_0 q_y(2q_x^2 + q_y^2)]\theta$ in the concentration equation. However, this does not modify the hydrodynamic mode structure to $\mathcal{O}(q_\perp)$ which is the focus of the paper and hence doesn't affect the long-time, large-distance theory of the polar phase described here.

## IV. ORDER ON A FLUCTUATING INTERFACE

Till now, I described the dynamics of uniaxial order at a perfectly flat interface. In this section, I consider apolar order at a fluctuating interface. For simplicity, I only consider the case in which the concentration of active nematogens *at the interface* is not conserved in which case I showed that long range nematic order is possible on a flat interface. I further assume that the order is strictly confined to the tangent plane and that the fluctuations of the interface are small. Therefore, I use the Monge gauge to parametrise the membrane displacement away from the $z = 0$ plane; that is, a point on the interface is parametrised by the three-dimensional position vector $\mathbf{R} = (x, y, h(x, y))$. With this parametrisation, the normal to the interface is $\mathbf{N} = \frac{\hat{z} - \nabla_\perp h}{\sqrt{1+(\nabla_\perp h)^2}}$. The three component nematic director, with in plane order along $\hat{x}$, is denoted by $\mathbf{n}(\mathbf{r}_\perp, t) \equiv (n_x, n_y, n_z) = \frac{\hat{x}+\delta\mathbf{n}}{\sqrt{1+\delta\mathbf{n}\cdot\delta\mathbf{n}}}$. Since the director is confined to the tangent plane,

$$\mathbf{n}\cdot\mathbf{N} = 0 = \frac{1}{\sqrt{1+\delta\mathbf{n}\cdot\delta\mathbf{n}}}\frac{1}{\sqrt{1+(\nabla_\perp h)^2}}[\delta n_z - \delta n_y\partial_y h - (1+\delta n_x)\partial_x h] \implies \delta n_z \approx \partial_x h \tag{87}$$

where the final approximate equality is obtained by retaining only the linear terms. The interface fluctuations are controlled by a free energy of the form

$$F_{\text{int}} = \frac{1}{2}\int d\mathbf{x}[\varsigma(\nabla_\perp h)^2 + \kappa(\nabla_\perp^2 h)^2] \tag{88}$$

where $\varsigma$ is the surface tension and $\kappa$ is the bending modulus. Denoting $\delta n_y = \theta$ for continuity of notation, the active force $\propto \nabla_\perp\cdot(\mathbf{nn}) = \partial_y\theta\hat{x} + \partial_x\theta\hat{y} + \partial_x^2 h\hat{z}$, to linear order, where I have used $\delta n_z \approx \partial_x h$. Putting all these together, the linearised force balance equation is

$$\eta\nabla^2\mathbf{V} = \nabla\Pi + \zeta(\partial_y\theta\hat{x} + \partial_x\theta\hat{y})\delta(z) + \left(\zeta\partial_x^2 h + \frac{\delta F_{\text{int}}}{\delta h}\right)\hat{z}\delta(z) + \boldsymbol{\xi}^v, \tag{89}$$

while the equation of motion for $\theta$ remains the same

$$\partial_t\theta = \Omega_{xy} - \lambda\cos 2\theta A_{xy} + \frac{\lambda}{2}\sin 2\theta(A_{xx} - A_{yy}) + \Gamma_\theta K\nabla_\perp^2\theta, \tag{90}$$

and that for the height fluctuations is simply

$$\partial_t h = v_z \tag{91}$$

where, as earlier, $v_z = V_z(z=0)$. Solving for the velocity fields, I get

$$v_x = \int_{-\infty}^{\infty} \frac{dq_z}{2\pi}\frac{i\zeta}{\eta q^4} q_y(q_x^2 - q_y^2 - q_z^2)\theta + \int_{-\infty}^{\infty}\frac{dq_z}{2\pi}\frac{1}{\eta q^4} q_x q_z(\varsigma q_\perp^2 + \kappa q_\perp^4 - \zeta q_x^2)h + \int_{-\infty}^{\infty}\frac{dq_z}{2\pi}\frac{1}{\eta q^4}[q_x(\xi_y^v q_y + \xi_z^v q_z) - \xi_x^v(q_y^2 + q_z^2)]$$
$$= -\frac{i\zeta}{2\eta}\frac{q_y^3}{|q_\perp|^3}\theta + \bar{\xi}_x^v, \tag{92}$$

$$v_y = \int_{-\infty}^{\infty} \frac{dq_z}{2\pi}\frac{i\zeta}{\eta q^4} q_x(q_y^2 - q_x^2 - q_z^2)\theta + \int_{-\infty}^{\infty}\frac{dq_z}{2\pi}\frac{1}{\eta q^4} q_y q_z(\varsigma q_\perp^2 + \kappa q_\perp^4 - \zeta q_x^2)h + \int_{-\infty}^{\infty}\frac{dq_z}{2\pi}\frac{1}{\eta q^4}[q_y(\xi_x^v q_x + \xi_z^v q_z) - \xi_y^v(q_x^2 + q_z^2)]$$
$$= -\frac{i\zeta}{2\eta}\frac{q_x^3}{|q_\perp|^3}\theta + \bar{\xi}_y^v \tag{93}$$

and

$$v_z = \int_{-\infty}^{\infty} \frac{dq_z}{2\pi}\frac{2i\zeta}{\eta q^4} q_x q_y q_z\theta - \int_{-\infty}^{\infty}\frac{dq_z}{2\pi}\frac{q_\perp^2}{\eta q^4}(\varsigma q_\perp^2 + \kappa q_\perp^4 - \zeta q_x^2)h + \int_{-\infty}^{\infty}\frac{dq_z}{2\pi}\frac{1}{\eta q^4}[q_z(\xi_x^v q_x + \xi_y^v q_y) - \xi_z^v q_\perp^2]$$
$$= -\frac{1}{4\eta|q_\perp|}(\varsigma q_\perp^2 + \kappa q_\perp^4 - \zeta q_x^2)h + \bar{\xi}_z^v. \tag{94}$$

As expected, $v_x$ and $v_y$ remain unchanged due to the fluctuations of the interface, but non-stochastic part of $v_z$ no longer vanishes. Therefore, the equation for angular fluctuations is still given by (24), i.e., to linear order, it is unaffected by the height fluctuations. while the linearised equation for the height fluctuations is

$$\partial_t h = -\frac{1}{4\eta|q_\perp|}(\varsigma q_\perp^2 + \kappa q_\perp^4 - \zeta q_x^2)h + \bar{\xi}_z^v, \tag{95}$$

i.e., activity yields an effective surface tension like term for fluctuations along the ordering direction. Therefore, the flat interface is destabilised for $\zeta > \varsigma$ i.e. when *extensile* activity is greater than the surface tension. In that case, the interface may have an undulated conformation as in [15] (note that the bending modulus also gets renormalised due to passive nematic elasticity [15]). This situation would generically be realised for an ordered phase on a self-assembled, tension-free membrane. The theory presented in the main text remains unchanged for interfaces for which $\zeta < \varsigma$ i.e., when the anisotropic effective surface tension is positive in all directions. In this case, the static structure factor of height fluctuations is

$$\langle |h(\mathbf{q}_\perp, t)|^2\rangle = \frac{\Delta^v}{\eta(\varsigma q_\perp^2 + \kappa q_\perp^4 - \zeta q_x^2)}. \tag{96}$$

The orientational order on this fluctuating interface will be described by the theory presented in this paper.

---

* nyomaitra07@gmail.com


[1] H. Stark, T. C. Lubensky, Phys. Rev. E **67**, 061709 (2003)
[2] D. Forster, Phys. Rev. Lett. **32**, 1161 (1974)
[3] A. Maitra, R. Voituriez, Phys. Rev. Lett. **124**, 048003 (2020)
[4] S Ramaswamy, RA Simha, J Toner, Europhys. Lett. **62**, 196 (2003)
[5] S. Ostlund, J. Toner, A. Zippelius, Ann. Phys. **144**, 345 (1982)
[6] R. A. Simha, S. Ramaswamy, Phys. Rev. Lett. **89**, 058101 (2002)
[7] G. Salbreux, J. Prost, J-F. Joanny, Phys. Rev. Lett 103, 058102 (2009)
[8] B. Martínez-Prat et al., Nat. Phys. **15**, 362 (2019)
[9] T. Gao et al., Phys. Rev. E **92**, 062709 (2015)
[10] T. Gao et al., Phys. Rev. Lett. **114**, 048101 (2015)
[11] M. C. Marchetti et al., Rev. Mod. Phys **85**, 1143 (2013)
[12] S. Ramaswamy, Annu. Rev. Condens. Matter Phys., **1**, 323 (2010)

[13] J. Toner and Y. Tu, Phys. Rev. Lett. **75**, 4326 (1995)
[14] J. Toner, Phys. Rev. E **86**, 031918 (2013)
[15] A. Senoussi et al., Proc. Natl. Acad. of Sci. **116**, 22464 (2019)
[16] J. Toner, Phys. Rev. Lett **108**, 088102 (2012)
[17] P. G. Saffman, M. Delbrück, Proc. Natl. Acad. Sci. USA **72**, 3111 (1975)
[18] P. M. Chaikin, T. C. Lubensky, Principles of Condensed Matter Physics, Cambridge University Press (2000)
[19] S. V. Maleev, Zh. Eksp. Teor. Fiz. **70**, 237 (1976)
[20] P. G. Maier, F. Schwabl, Phys. Rev. B **70**, 134430 (2004)
[21] R. A. Pelcovits, B. I. Halperin, Phys. Rev. B **19**, 4614 (1979)
[22] T. Sanchez et al., Nature **491**, 431 (2012)
[23] P. Guillamat et al. Phys. Rev. E **94**, 060602 (2016)
[24] A. Maitra et al., Phys. Rev. Lett. **124**, 028002 (2020)
[25] S. Shankar et al., Phys. Rev. Lett. **121**, 10800 (2018)
[26] A. Maitra, M. Lenz, R. Voituriez, Phys. Rev. Lett. **125**, 238005 (2020)
[27] F. Vafa et al., arXiv: 2007.02947 (2020)
[28] L. Angheluta et al., arXiv: 2012.02980 (2020)
